# Supplementary material for: WearableMil: An End-to-End Framework for Military Activity Recognition and Performance Monitoring
Source: arXiv:2410.05452 source file (2025-04-28)
Supplement: Supplementary file 1 [file appendix.tex]

\begin{table*}[h!]
\centering
\begin{tabular}{|c|c|c|c|c|c|c|}\hline
\textbf{User ID} & \textbf{Total Before} & \textbf{Total After} & \textbf{Difference} & \textbf{Reason 1} & \textbf{Reason 2} & \textbf{Reason 3} \\ \hline
1 & 5586 & 9745 & 4159 & 242 & 3915 & 2 \\ 
2 & 173171 & 258807 & 85636 & 5470 & 80117 & 49 \\ 
3 & 6033 & 9900 & 3867 & 316 & 3549 & 2 \\ 
4 & 45378 & 106276 & 60898 & 3982 & 56873 & 43 \\ 
5 & 69739 & 105176 & 35437 & 1373 & 34044 & 20 \\ 
6 & 17218 & 28790 & 11572 & 286 & 11284 & 2 \\ 
7 & 8584 & 21260 & 12676 & 413 & 12258 & 5 \\ 
8 & 95323 & 144380 & 49057 & 2703 & 46326 & 28 \\ 
9 & 99424 & 151931 & 52507 & 1963 & 50514 & 30 \\ 
10 & 121436 & 189236 & 67800 & 5120 & 62630 & 50 \\ 
11 & 63863 & 107411 & 43548 & 2103 & 41428 & 17 \\ 
12 & 41446 & 98822 & 57376 & 2472 & 54879 & 25 \\ 
13 & 11303 & 23372 & 12069 & 810 & 11254 & 5 \\ 
14 & 246116 & 353218 & 107102 & 7209 & 99837 & 56 \\ 
15 & 45255 & 78072 & 32817 & 2181 & 30610 & 26 \\ 
16 & 12548 & 28348 & 15800 & 402 & 15396 & 2 \\ 
17 & 0 & 342 & 342 & 141 & 201 & 0 \\ 
18 & 20363 & 34505 & 14142 & 914 & 13213 & 15 \\ 
19 & 7622 & 12543 & 4921 & 220 & 4699 & 2 \\ 
20 & 0 & 2686 & 2686 & 265 & 2421 & 0 \\ 
21 & 152523 & 210470 & 57947 & 2950 & 54979 & 18 \\ 
22 & 18763 & 29939 & 11176 & 590 & 10579 & 7 \\ 
23 & 40882 & 67828 & 26946 & 1381 & 25553 & 12 \\ 
24 & 0 & 2 & 2 & 2 & 0 & 0 \\ 
25 & 211140 & 303819 & 92679 & 5146 & 87480 & 53 \\ 
26 & 0 & 2174 & 2174 & 312 & 1862 & 0 \\ 
27 & 150765 & 215891 & 65126 & 3118 & 61967 & 41 \\ 
28 & 77690 & 162871 & 85181 & 5078 & 80048 & 55 \\ 
29 & 237022 & 348579 & 111557 & 6860 & 104642 & 55 \\ 
30 & 129782 & 211958 & 82176 & 3847 & 78292 & 37 \\ 
31 & 328 & 2551 & 2223 & 135 & 2088 & 0 \\ 
32 & 138328 & 224572 & 86244 & 4426 & 81782 & 36 \\ 
33 & 0 & 9 & 9 & 0 & 9 & 0 \\ 
34 & 2013 & 3285 & 1272 & 43 & 1229 & 0 \\ 
35 & 27656 & 50754 & 23098 & 1149 & 21935 & 14 \\ 
36 & 20979 & 41147 & 20168 & 1395 & 18754 & 19 \\ 
37 & 30432 & 80011 & 49579 & 3205 & 46366 & 8 \\ 
38 & 84920 & 128852 & 43932 & 1946 & 41966 & 20 \\ 
39 & 116396 & 166525 & 50129 & 1571 & 48537 & 21 \\ 
40 & 54732 & 83476 & 28744 & 851 & 27882 & 11 \\ 
41 & 116570 & 170477 & 53907 & 2757 & 51131 & 19 \\ 
42 & 16941 & 23439 & 6498 & 420 & 6075 & 3 \\ 
43 & 17658 & 45388 & 27730 & 715 & 27003 & 12 \\ 
44 & 80190 & 131711 & 51521 & 2873 & 48626 & 22 \\ 
45 & 83625 & 134398 & 50773 & 1700 & 49052 & 21 \\ 
46 & 125696 & 202302 & 76606 & 5085 & 71469 & 52 \\ 
47 & 7292 & 12799 & 5507 & 407 & 5097 & 3 \\ 
48 & 0 & 2 & 2 & 0 & 2 & 0 \\ 
49 & 143094 & 216598 & 73504 & 4521 & 68933 & 50 \\ 
50 & 0 & 2417 & 2417 & 198 & 2219 & 0 \\ 
\hline
\end{tabular}
\caption{Detailed statistics for the first 50 users, including the total before and after imputation, differences, and reasons for the imputed values.}
\label{tab:user_statistics_1}
\end{table*}

\begin{table*}[h!]
\centering
\begin{tabular}{|c|c|c|c|c|c|c|}
\hline
\textbf{User ID} & \textbf{Total Before} & \textbf{Total After} & \textbf{Difference} & \textbf{Reason 1} & \textbf{Reason 2} & \textbf{Reason 3} \\ 
\hline
51 & 102124 & 165686 & 63562 & 4088 & 59421 & 53 \\ 
52 & 0 & 2955 & 2955 & 296 & 2659 & 0 \\ 
53 & 0 & 869 & 869 & 111 & 758 & 0 \\ 
54 & 137911 & 211457 & 73546 & 4429 & 69076 & 41 \\ 
55 & 106673 & 168168 & 61495 & 3484 & 57978 & 33 \\ 
56 & 870 & 5662 & 4792 & 187 & 4604 & 1 \\ 
57 & 0 & 1681 & 1681 & 60 & 1621 & 0 \\ 
58 & 7039 & 24323 & 17284 & 1512 & 15772 & 0 \\ 
59 & 104672 & 187812 & 83140 & 4483 & 78616 & 41 \\ 
60 & 13511 & 19874 & 6363 & 624 & 5733 & 6 \\ 
61 & 31001 & 86126 & 55125 & 4178 & 50910 & 37 \\ 
62 & 19773 & 90538 & 70765 & 1752 & 69003 & 10 \\ 
63 & 51332 & 93035 & 41703 & 2352 & 39326 & 25 \\ 
64 & 1289 & 3411 & 2122 & 191 & 1931 & 0 \\ 
65 & 196472 & 273442 & 76970 & 5076 & 71845 & 49 \\ 
66 & 79211 & 122563 & 43352 & 1478 & 41847 & 27 \\ 
67 & 228100 & 365534 & 137434 & 10676 & 126687 & 71 \\ 
68 & 26973 & 74334 & 47361 & 3110 & 44214 & 37 \\ 
69 & 34533 & 41142 & 6609 & 562 & 6040 & 7 \\ 
70 & 7002 & 17031 & 10029 & 370 & 9656 & 3 \\ 
71 & 0 & 968 & 968 & 91 & 877 & 0 \\ 
72 & 535 & 11585 & 11050 & 325 & 10725 & 0 \\ 
73 & 78523 & 138581 & 60058 & 2351 & 57682 & 25 \\ 
74 & 186502 & 322476 & 135974 & 7572 & 128325 & 77 \\ 
75 & 1350 & 4470 & 3120 & 237 & 2881 & 2 \\ 
76 & 279725 & 370231 & 90506 & 6690 & 83769 & 47 \\ 
77 & 11484 & 20586 & 9102 & 447 & 8649 & 6 \\ 
78 & 7861 & 14033 & 6172 & 447 & 5723 & 2 \\ 
79 & 68755 & 113363 & 44608 & 2138 & 42446 & 24 \\ 
80 & 219588 & 306091 & 86503 & 4972 & 81462 & 69 \\ 
81 & 90501 & 132598 & 42097 & 1878 & 40186 & 33 \\ 
82 & 30793 & 51681 & 20888 & 1427 & 19454 & 7 \\ 
83 & 107604 & 153974 & 46370 & 1470 & 44872 & 28 \\ 
84 & 67222 & 109769 & 42547 & 2632 & 39884 & 31 \\ 
85 & 139217 & 216564 & 77347 & 3849 & 73467 & 31 \\ 
86 & 18447 & 28879 & 10432 & 604 & 9823 & 5 \\ 
87 & 3552 & 12973 & 9421 & 974 & 8443 & 4 \\ 
88 & 63119 & 95366 & 32247 & 949 & 31289 & 9 \\ 
89 & 11540 & 23038 & 11498 & 658 & 10831 & 9 \\ 
90 & 20631 & 20978 & 347 & 43 & 304 & 0 \\ 
91 & 12000 & 24861 & 12861 & 750 & 12107 & 4 \\ 
92 & 190870 & 275831 & 84961 & 4661 & 80262 & 38 \\ 
93 & 106487 & 201468 & 94981 & 6751 & 88179 & 51 \\ 
94 & 4487 & 15039 & 10552 & 422 & 10128 & 2 \\ 
95 & 20769 & 48868 & 28099 & 1527 & 26554 & 18 \\ 
96 & 58359 & 112818 & 54459 & 6082 & 48325 & 52 \\ 
97 & 110363 & 171143 & 60780 & 3303 & 57455 & 22 \\ 
98 & 8526 & 15803 & 7277 & 261 & 7015 & 1 \\ 
99 & 0 & 89 & 89 & 15 & 74 & 0 \\ 
100 & 43254 & 96255 & 53001 & 4209 & 48766 & 26 \\ 
\hline
\end{tabular}
\caption{Detailed statistics for the next 50 users, including the total before and after imputation, differences, and reasons for the imputed values.}
\label{tab:user_statistics_2}
\end{table*}

\begin{table*}[h!]
\centering
\begin{tabular}{|c|c|c|c|c|c|c|}
\hline
\textbf{User ID} & \textbf{Total Before} & \textbf{Total After} & \textbf{Difference} & \textbf{Reason 1} & \textbf{Reason 2} & \textbf{Reason 3} \\ 
\hline
101 & 99273 & 363833 & 264560 & 23567 & 240908 & 85 \\ 
102 & 46389 & 82295 & 35906 & 1493 & 34403 & 10 \\ 
103 & 293063 & 395012 & 101949 & 6421 & 95466 & 62 \\ 
104 & 66955 & 95698 & 28743 & 1286 & 27442 & 15 \\ 
105 & 81885 & 106976 & 25091 & 1760 & 23320 & 11 \\ 
106 & 4667 & 8307 & 3640 & 193 & 3445 & 2 \\ 
107 & 15305 & 30426 & 15121 & 425 & 14691 & 5 \\ 
108 & 184123 & 290552 & 106429 & 6109 & 100265 & 55 \\ 
109 & 245682 & 345336 & 99654 & 6082 & 93505 & 67 \\ 
110 & 126848 & 225380 & 98532 & 5445 & 93038 & 49 \\ 
111 & 50946 & 118859 & 67913 & 3003 & 64886 & 24 \\ 
112 & 447 & 3776 & 3329 & 45 & 3284 & 0 \\ 
113 & 981 & 5214 & 4233 & 478 & 3751 & 4 \\ 
114 & 229938 & 333485 & 103547 & 4720 & 98771 & 56 \\ 
115 & 30004 & 52855 & 22851 & 582 & 22259 & 10 \\ 
116 & 45254 & 68504 & 23250 & 1354 & 21884 & 12 \\ 
117 & 0 & 1493 & 1493 & 165 & 1328 & 0 \\ 
118 & 3084 & 6893 & 3809 & 206 & 3601 & 2 \\ 
119 & 152981 & 209509 & 56528 & 3110 & 53373 & 45 \\ 
120 & 162427 & 252647 & 90220 & 7791 & 82363 & 66 \\ 
121 & 11894 & 94280 & 82386 & 8608 & 73776 & 2 \\ 
122 & 49869 & 83051 & 33182 & 1714 & 31451 & 17 \\ 
123 & 135682 & 211195 & 75513 & 3828 & 71635 & 50 \\ 
124 & 75013 & 137418 & 62405 & 3192 & 59182 & 31 \\ 
125 & 6836 & 34649 & 27813 & 683 & 27129 & 1 \\ 
126 & 26214 & 45100 & 18886 & 1166 & 17705 & 15 \\ 
127 & 74276 & 132564 & 58288 & 3698 & 54551 & 39 \\ 
128 & 9091 & 16208 & 7117 & 218 & 6894 & 5 \\ 
129 & 141161 & 215514 & 74353 & 2678 & 71624 & 51 \\ 
130 & 2496 & 10461 & 7965 & 583 & 7379 & 3 \\ 
131 & 51585 & 142886 & 91301 & 6437 & 84815 & 49 \\ 
132 & 66691 & 81510 & 14819 & 1094 & 13711 & 14 \\ 
133 & 11326 & 17990 & 6664 & 386 & 6277 & 1 \\ 
134 & 13814 & 19477 & 5663 & 368 & 5294 & 1 \\ 
135 & 20084 & 36679 & 16595 & 1044 & 15545 & 6 \\ 
\hline
\end{tabular}
\caption{Detailed statistics for the next remaining users, including the total before and after imputation, differences, and reasons for the imputed values.}
\label{tab:user_statistics_3}
\end{table*}
